# Supplementary material for: Robust Testing in High-Dimensional Sparse Models
Source: arXiv:2205.07488 source file (2022-11-04)
Supplement: Supplementary file 1 [file APPENDICES.tex]

\appendix
\section{Sparse Gaussian mean testing}\label{sec:SGMT}
In this section we provide a proof of the lower bound on the sample complexity of sparse Gaussian mean testing. Define the function $N$ as 
\begin{equation}\label{eqn:smt_sampleCxty}
N(s,d,\gamma)=\begin{cases}
			\frac{s}{\gamma^2}\log\left(1+\frac{d}{s^2}\right) & \text{if  }s<\sqrt{d}\\
            \frac{\sqrt{d}}{\gamma^2} & \text{if  }s\ge \sqrt{d}
		 \end{cases}.    
\end{equation}
\begin{proposition}\label{prop:smt}
Let $\gamma>0$ be fixed. Let $X_1,X_2,\cdots,X_n$ be i.i.d. samples from a distribution $\p$. Then, any algorithm that distinguishes between the cases $\p=\cN(0,I_d)$ and $\p\in\{\cN(\theta,I_d):\normtwo{\theta}\ge\gamma,\norm{\theta}_0\le s\}$ with probability greater than $2/3$ requires $n\ge cN(s,d,\gamma)$, where $N$ is given by (\ref{eqn:smt_sampleCxty}) and $c$ is constant.
\end{proposition}
\begin{proof}
Let $B=\{b\in\{0,1\}^d:\norm{b}_0=s\}$ and $b\sim\text{Uniform}(B)$. Let $\Theta = \frac{\gamma }{\sqrt{s}}B$. With $\q_\theta=\cN(\theta,I_d)$ and $\q=\bE{\theta}{\q_\theta}$, by (\ref{eqn:chi2_div}) we have
\begin{align*}
    1+\chisquare{\q}{G^n} = \bE{\theta,\theta'}{\left(1+\chi^2_{G}(\q_\theta,\q_{\theta'})\right)^n}.
\end{align*}
Since $\q_\theta = \mathcal{N}(\theta,I_d)$, a straightforward computation gives
\begin{equation*}
    1+\chi^2_{G}(\q_\theta,\q_{\theta'}) = \exp(\langle\theta,\theta'\rangle).
\end{equation*}
Thus,
\begin{align*}
    1+\chisquare{\q}{G^n} &= \bE{\theta,\theta'}{\exp(n\langle\theta,\theta'\rangle)}\\
    &= \bE{b,b'}{\exp\left(\frac{n\gamma^2}{s}\langle b,b'\rangle\right)}.
\end{align*}    
By symmetry between $b$ and $b'$ in the above equation, it suffices to evaluate the expectation keeping $b'$ fixed, say at $b_0$. Then the $\langle b,b_0\rangle$ has Hypergeometric distribution. Hence,
\begin{align*}
    1+\chisquare{\q}{G^n} &= \bE{b}{\exp\left(\frac{n\gamma^2}{s}\langle b,b_0\rangle\right)}\\
    &= \expect{\exp\left(\frac{n\gamma^2}{s}H\right)},
\end{align*}
where $H\sim\hypergeom(d,s,s)$. Let $B\sim$Binomial$(s,\frac{s}{d})$. Then by Theorem~23.1 in \cite{Wu20}, we have
\begin{equation*}
    \expect{\exp(\lambda H)}\le \expect{\exp(\lambda B)} = \left(1+\frac{s}{d}(e^\lambda-1)\right)^s.
\end{equation*}
Thus,
\begin{align*}
    \chisquare{\q}{G^n} &\le \left(1+\frac{s}{d}(e^{\frac{n\gamma^2}{s}}-1)\right)^s-1\\
    &\le \exp\left(\frac{s^2}{d}(e^{\frac{n\gamma^2}{s}}-1)\right)-1.
\end{align*}
Therefore, for $\chisquare{\q}{G^n}$ to be $\Omega(1)$, we need $n=\Omega\left(\frac{s}{\gamma^2}\log\left(1+\frac{d}{s^2}\right)\right)$. For $s=\sqrt{d}$, we get $n=\Omega\left(\frac{\sqrt{d}}{\gamma^2}\right)$. By construction, the sample complexity at lower values of $s$ is a lower bound for higher values of $s$. Hence, we have $n=\Omega\left(\frac{\sqrt{d}}{\gamma^2}\right)$ for $s\ge\sqrt{d}$.   
\end{proof}
\begin{remark}
The sample complexity in Proposition~\ref{prop:smt} turns out to be tight. Let $\hat{\theta}\eqdef \frac{1}{n}\sum_{i=1}^n X_i$ and $\alpha \eqdef \expectCond{Y^2}{Y^2>\beta^2}$, where $Y\sim \cN(0,1)$ and $\beta = \sqrt{2\log(1+d/s^2)}$. Define the statistic $\hat{T}$ as $\hat{T} = \sqrt{\max\{\hat{S},0\}}$, where 
\begin{equation*}
    \hat{S} = \begin{cases}
			\sum_{j=1}^d (\hat{\theta}_j^2-\alpha/n)\mathds{1}_{\left\{|\hat{\theta}_j|>
			\frac{\beta}{\sqrt{n}}\right\}} & \text{if  }s<\sqrt{d}\\
            	\sum_{j=1}^d \hat{\theta}_j^2-d/n & \text{if  }s\ge \sqrt{d}
		 \end{cases}.  
\end{equation*}
The test $\hat{T}\ge\gamma/2$ achieves the lower bound given in Proposition~\ref{prop:smt} \cite{Olivier17}.
\end{remark}
